# Supplementary material for: Precise prediction of the decay rate for $\eta_b\to \gamma \gamma$ from lattice QCD
Source: arXiv:2410.24041 ancillary file (2025-12-18)
Supplement: Supplementary file 1 [file supplementary_materials.pdf]

## SUPPLEMENTARY MATERIALS

### THE LATTICE CALCULATION

On each set of gluon field configurations we tune the valence quark mass in lattice units so that the heavyonium pseudoscalar meson takes the value of the experimental mass of the  $\eta_b$  meson, 6.62 GeV or 4.0 GeV, as explained in the main text. This tuning is done using the ‘Goldstone’ (spin-taste  $\gamma_5 \otimes \gamma_5$ ) meson. For the three-point correlation functions we use the spin-taste  $\gamma_5 \gamma_t \otimes \gamma_x \gamma_z$  operator to project onto the heavyonium pseudoscalar meson since this allows us to use two local vector currents to couple to the two photons. The mass of the ground-state pseudoscalar meson for this second spin-taste has a slightly heavier mass than the Goldstone meson because of staggered quark discretisation effects. We also determine the mass of this non-Goldstone meson and use it to fix the (equal and opposite) spatial momentum that we give to the two photons; each is given a momentum equal to half the mass for the on-shell condition to hold. We take the momentum to be in the  $y$ -direction, orthogonal to the polarisations of both vector currents. The momentum is inserted using twisted boundary conditions and the twist angles are listed in Table I.

TABLE I. Twists,  $\theta$ , used for the sequential propagator for the three heavyonium pseudoscalar meson masses (for the ‘Goldstone’ spin-taste) listed in the first row. The twist was taken in the  $y$ -direction and the corresponding 3-momentum component is given by  $q^y = \theta\pi/L_s$ . Also listed, in the final column, are the  $T$  values in lattice units for the temporal axial current operator relative to the origin position of the first vector current operator (see Figure 1 in the main text).

|         |          | Twist, $\theta$ |         | $T/a$                           |
|---------|----------|-----------------|---------|---------------------------------|
| Set     | $\eta_b$ | 6.62 GeV        | 4.0 GeV |                                 |
| c-5     |          |                 | 9.7627  | 7, 10, 13, 16, 19, 22           |
| c-phys  |          |                 | 19.1217 | 7, 10, 13, 16, 19, 22           |
| f-5     |          | 15.5890         | 9.3123  | 9, 12, 15, 18, 21               |
| f-phys  |          | 30.5000         | 18.2490 | 9, 12, 15, 18, 21               |
| sf-5    | 21.5873  | 15.1834         | 9.1832  | 14, 17, 22, 25, 30 <sup>a</sup> |
| sf-phys | 41.5678  | 29.1932         |         | 12, 17, 22, 27, 32, 37          |
| uf-5    | 21.3832  | 14.6348         |         | 22, 29, 36, 43                  |
| ef-5    | 23.8113  | 16.8212         |         | 21, 30, 39, 48, 57 <sup>b</sup> |

<sup>a</sup> For the  $am_h = 0.412$  ( $M_{\eta_h} = 4$  GeV) case the  $T/a$  values were 12, 17, 22, 27, 32, 37

<sup>b</sup>  $T/a = 57$  was used for the  $am_h = 0.403$  ( $M_{\eta_h} = 6.62$  GeV) case only.

We also list in Table I the values of  $T/a$  used in our three-point correlation functions, on each set of gluon field configurations.  $T$  is the time separation between one of the vector operators (positioned at the origin) and the temporal axial current. Multiple  $T$  values are used; these are the values at which the two-point function  $\tilde{C}$ , resulting from a weighted sum over the three-point function, is

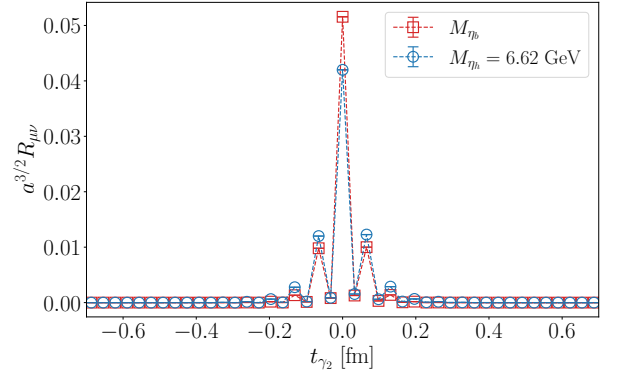

FIG. 1. Normalised summand,  $R_{\mu\nu}$ , defined in Eq. (1), for two different masses on the ef-5 gluon field ensemble. The meson masses correspond to the  $\eta_b$  mass (open red squares) and 6.62 GeV (open blue circles).  $T = 21$  here, corresponding to 0.69 fm, well outside the region where  $R_{\mu\nu}$  is significantly different from zero.

sampled. The normalised summand,  $R_{\mu\nu}$ , for the  $\eta_b$  case on the ef-5 lattices is shown in Figure 1 as a function of the time separation between the two vector current operators.  $R_{\mu\nu}$  is defined as [1]:

$$R_{\mu\nu}(t_{\gamma_2}) = \frac{e^{-\omega t_{\gamma_2}} C_{3\text{pt}}(0, t_{\gamma_2}, T)}{a_0 e^{-M_{\eta_h}(T-t_{\gamma_2})}}, \quad (1)$$

where  $C_{3\text{pt}}$  is the three-point correlation function shown schematically in Figure 1 of the main text. The denominator of the ratio is obtained from the two-point correlation function and removes the exponential time dependence for clarity. We see that the summand peaks when the two vector current operators are close in time, and falls off rapidly on either side of this point. We choose  $T$  values so that the temporal axial current operator is well outside the region of this peak, which means that the resulting two-point function,  $\tilde{C}(T)$ , projects well onto the ground-state pseudoscalar meson. By fitting  $\tilde{C}(T)$  and the two-point function for the temporal axial current,  $C(t)$ , simultaneously to a multi-exponential form we can determine the amplitude for the pseudoscalar meson to decay to two on-shell photons (see Eq. (4) of the main text).

Tables II and III give the Goldstone and non-Goldstone pseudoscalar meson masses on each ensemble and for each value of  $am_h$  from our fits. Table IV gives the corresponding values for  $R_{\eta_h}$ , defined in Eq. (2) of the main text as the ratio of decay constant to form factor times mass-squared. The Goldstone  $\eta_h$  is the one that appears in the decay constant calculation and the non-Goldstone  $\eta_h$  appears in the  $\eta_h \rightarrow \gamma\gamma$  form factor calculation. They differ by discretisation effects that vanish in the continuum limit and a comparison of Tables II and III shows the differences to be very small on all ensembles.

TABLE II. Values for the mass of the Goldstone  $\eta_h$  on each ensemble.

| Ensemble | $aM_{\eta_h}(\gamma_5 \otimes \gamma_5)$ |              |              |
|----------|------------------------------------------|--------------|--------------|
|          | $\eta_b$                                 | 6.62 GeV     | 4 GeV        |
| c-5      | -                                        | -            | 2.529041(34) |
| c-phys   | -                                        | -            | 2.478803(17) |
| f-5      | -                                        | 3.021819(33) | 1.824274(64) |
| f-phys   | -                                        | 2.961363(20) | 1.787579(37) |
| sf-5     | 2.825095(14)                             | 1.987492(23) | 1.201411(42) |
| sf-phys  | 2.713642(12)                             | 1.909183(18) | -            |
| uf-5     | 2.098210(17)                             | 1.436342(24) | -            |
| ef-5     | 1.558192(25)                             | 1.101002(31) | -            |

TABLE III. Values for the mass of the non-Goldstone  $\eta_h$  on each ensemble for each choice of (Goldstone)  $M_{\eta_h}$ .

| Ensemble | $aM_{\eta_h}(\gamma_5 \gamma_t \otimes \gamma_x \gamma_z)$ |              |              |
|----------|------------------------------------------------------------|--------------|--------------|
|          | $\eta_b$                                                   | 6.62 GeV     | 4 GeV        |
| c-5      | -                                                          | -            | 2.555920(59) |
| c-phys   | -                                                          | -            | 2.502987(34) |
| f-5      | -                                                          | 3.06087(11)  | 1.828517(71) |
| f-phys   | -                                                          | 2.994337(54) | 1.791584(40) |
| sf-5     | 2.834564(20)                                               | 1.989187(25) | 1.202071(47) |
| sf-phys  | 2.720588(15)                                               | 1.910690(20) | -            |
| uf-5     | 2.099315(17)                                               | 1.436773(25) | -            |
| ef-5     | 1.558447(26)                                               | 1.101149(31) | -            |

TABLE IV. Values for  $R_{\eta_h}$  on each ensemble for each choice of (Goldstone)  $M_{\eta_h}$  mass. Results for  $\eta_h = \eta_c$  are given in [1] for a slightly different ratio.

| Ensemble | $R_{\eta_h}$ |              |              |
|----------|--------------|--------------|--------------|
|          | $\eta_b$     | 6.62 GeV     | 4 GeV        |
| c-5      | -            | -            | 0.63488(61)  |
| c-phys   | -            | -            | 0.62611(262) |
| f-5      | -            | 0.76127(183) | 0.51964(67)  |
| f-phys   | -            | 0.73980(84)  | 0.51908(42)  |
| sf-5     | 0.66818(59)  | 0.51761(54)  | 0.49452(76)  |
| sf-phys  | 0.63483(54)  | 0.51221(47)  | -            |
| uf-5     | 0.52372(120) | 0.49234(114) | -            |
| ef-5     | 0.48636(59)  | 0.48050(80)  | -            |

## RESULTS AND CONCLUSIONS

Chiral/continuum fits are carried out independently for each value of the  $\eta_h$  mass using the form given in Eq. (5) of the main text. Following [1] we take an Empirical Bayes approach to our fits, allowing the scale parameter  $\Lambda$  that appears in the first discretisation term to be adjusted such that it maximises the Bayes factor [2]. The final term also allows for discretisation errors from the sea quarks. Here we set  $\tilde{\Lambda} = 1$  GeV.

We include  $\delta$  terms in our fit form that allow for the mistuning of sea and valence quark masses. These are

taken to be:

$$\delta^{\text{val},h} = \frac{am_h^{\text{val}} - am_h^{\text{tuned}}}{am_h^{\text{tuned}}}, \quad (2)$$

$$\delta^{\text{sea},c} = \frac{am_c^{\text{sea}} - am_c^{\text{tuned}}}{am_c^{\text{tuned}}}, \quad (3)$$

$$\delta^{\text{sea},uds} = \frac{2am_l^{\text{sea}} + am_s^{\text{sea}} - 2am_l^{\text{tuned}} - am_s^{\text{tuned}}}{10am_s^{\text{tuned}}}. \quad (4)$$

The heavy quark mass is tuned by

$$am_h^{\text{tuned}} = am_h^{\text{val}} \left( \frac{M_{\eta_h}^{\text{phys}}}{M_{\eta_h}} \right)^{1.5}, \quad (5)$$

where we take  $M_{\eta_h}^{\text{phys}}$  as the appropriate pseudoscalar mass:  $M_{\eta_b} = 9.3987$  GeV from experiment [3], or our intermediate values of 6.62 GeV or 4 GeV. The power is set as 1.5 based on empirical observation from charmium results [4].

The mass of the  $s$  quark is tuned through

$$am_s^{\text{tuned}} = am_s^{\text{val}} \left( \frac{M_{\eta_s}^{\text{phys}}}{M_{\eta_s}} \right)^2, \quad (6)$$

and  $am_l^{\text{tuned}}$  is determined using the ratio [5]

$$\frac{m_s^{\text{phys}}}{m_l^{\text{phys}}} = 27.18(10). \quad (7)$$

Tuned  $s$  quark masses are taken from Table V of [6] where available. For ensembles f-5 and uf-5 we use  $\eta_s$  masses from [7] alongside the ‘physical’  $\eta_s$  mass of 688.5(2.2) MeV [8] to tune the  $s$  quark using Eq. (6). We tuned the  $s$  quark from the ratio [9]

$$\frac{m_c}{m_s} = 11.783(25) \quad (8)$$

for the sf-p and ef-5 ensembles where we have not calculated  $M_{\eta_s}$ . All  $am_l^{\text{tuned}}$  values were determined from the tuned  $s$  quarks using Eq. (7).

For the fit priors we use  $R_{\eta_h}^{\text{phys}} = 0.5(2)$ ,  $\kappa_{a\Lambda}^{(i)} = 0(2)$ ,  $\kappa_{\text{sea},c} = 0.0(1)$  and  $\kappa_{\text{sea},uds}^{(i)} = 0(1)$ . The mistuning parameter corresponding to the heavy quark mass is set as  $\kappa_{\text{val},h} = 0.00(5)$  (since we know from [1] that  $R_{\eta_h}$  has little dependence on  $m_h$ ). Our preferred fit for each mass uses  $i_{\text{max}} = 5$  so that discretisation effects up to  $(\Lambda a)^{10}$  are included.

The  $\eta_b$  results and fit curve are shown in the main text. Here we show plots for the  $M_{\eta_h} = 6.62$  GeV and 4 GeV cases in Figures 2 and 3 respectively. Numerical values for  $R_{\eta_h}$  from our chiral/continuum fits are given in Table V along with the value of  $\Lambda$  chosen using the Empirical Bayes criterion. We also give an error budget from the fits.

In [1] we calculated  $f_{J/\psi}/(F(0,0)^2 M_{J/\psi}^2)$  at the  $\eta_c$  mass, obtaining  $0.4786(57)_{\text{fit}}(14)_{\text{syst}}$ . We can convert this result to the ratio  $R_{\eta_c}$  that we are using here by taking the value of  $f_{J/\psi}/f_{\eta_c}$  and the ‘connected’  $M_{\eta_c}$  from [4] alongside the experimental value of  $M_{J/\psi}$  [3]. This gives  $R_{\eta_c} = 0.5031(61)$ , which does not include the systematic error. To compare directly with our results at other masses here, we calculate  $R_{\eta_c}$  from the results of [1] (taking  $f_{\eta_c}$  and  $M_{\eta_c}$  directly from our simultaneous correlator fits) and perform a continuum/chiral fit at the  $\eta_c$  mass in the same way as for the other masses. Doing this, we find  $R_{\eta_c} = 0.5014(59)$ , in good agreement with the result above.

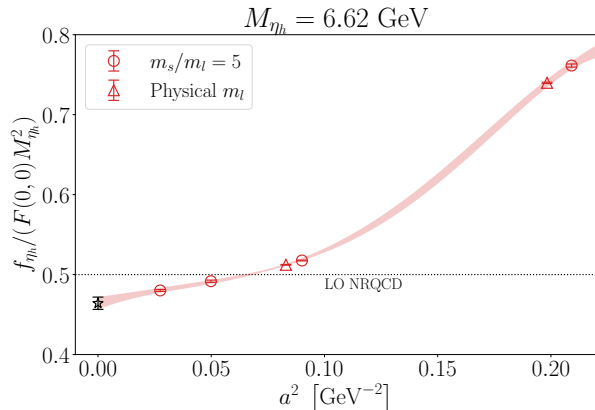

FIG. 2. Plot showing how the continuum/chiral limit is obtained for  $R_{\eta_h}$  for  $M_{\eta_h} = 6.62$  GeV. Lattice points are shown by the red circles and the fit by the red band. For the point on the uf-5 ensemble the valence mass was not as well tuned as elsewhere and we plot an adjusted value in which we use the output of the fit for the  $\delta^{\text{val},h}$  term to correct for the mistuning (the adjustment is barely visible). The result in the continuum limit is give by the black star. The leading order NRQCD expectation is depicted by the dotted line.

TABLE V. Results for  $R_{\eta_h}$  from the chiral/continuum fits for pseudoscalar mesons masses at the  $\eta_h$  masses  $M_{\eta_h}$ , 6.62 GeV and 4.0 GeV. We give the value of  $\Lambda$  obtained using the Empirical Bayes criterion. We also provide error budgets from the fits to  $R_{\eta_h}$ . Note that the valence quark on the uf-5 ensemble in the  $M_{\eta_h} = 6.62$  GeV case is not as well-tuned as elsewhere, leading to a larger contribution from the valence mistuning in the error budget.

|                       | $\eta_b$    | 6.62 GeV   | 4 GeV      |
|-----------------------|-------------|------------|------------|
| $R_{\eta_h}$          | 0.4682(108) | 0.4645(71) | 0.4988(97) |
| $\Lambda[\text{GeV}]$ | 2.422       | 2.237      | 1.104      |
| Statistics            | 0.76        | 0.98       | 0.54       |
| $w_0/a$               | 0.41        | 0.27       | 0.07       |
| $w_0$                 | 0.01        | 0.09       | 0.04       |
| $a^2 \rightarrow 0$   | 2.06        | 0.77       | 1.23       |
| Valence Mistuning     | 0.16        | 0.78       | 0.10       |
| Sea Mistuning         | 0.50        | 0.30       | 1.38       |
| Total (%)             | 2.29        | 1.53       | 1.93       |

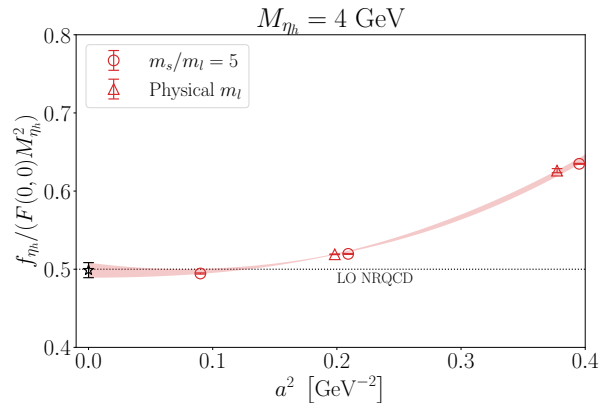

FIG. 3. Plot showing how the continuum/chiral limit is obtained for  $R_{\eta_h}$  for  $M_{\eta_h} = 4.0$  GeV. Lattice points are shown by the red circles and the fit by the red band. The result in the continuum limit is give by the black star. The leading order NRQCD expectation is depicted by the dotted line.

For our preferred fits we arranged the momentum entirely in the  $y$ -direction. However, only a component of the momentum need be orthogonal to the polarisations of the vector currents and the expectation is that this choice results in a difference in discretisation errors that vanish in the continuum limit. We check this by splitting the momentum over the three spatial directions equally on ensembles c-5, f-5 and sf-5 for an  $\eta_h$  with mass 4.0 GeV. Figure 4 compares the two approaches. The excellent agreement between the results in the continuum limit confirms that changing the momentum setup does indeed simply lead to a difference in discretisation effects. Note that since the 111-mom result only has data points for gluon field ensembles with  $m_s/m_l = 5$  it cannot capture the dependence on the light sea quark mass. We therefore set the prior on  $\kappa_{uds}^{(0)}$  to be equal to that of its posterior value from the preferred fit.

We checked the stability of our results for  $R_{\eta_h}$  by making variations to the correlator fits and to the chiral/continuum fits. The results of these checks for  $R_{\eta_b}$  are shown in Figure 5. The point labelled ‘base fit’ is our preferred result, which is also indicated by the horizontal band. We test the effects of both halving and doubling the prior widths on the parameters in the correlator fits and find almost no effect on the result. We similarly halve and double the prior widths on parameters in the chiral/continuum fit, which has a small effect well within the uncertainty of the base fit. Finally, we remove and add a  $\kappa_{a\Lambda}$  term in the fit form given in Eq. (5) of the main text. This shows virtually no difference between these variations and the base fit where  $i_{\text{max}} = 5$ , indicating that we have a suitable number of discretisation terms in the fit. We carry out the same checks for the other masses and find similarly good agreement. For  $M_{\eta_h} = 6.62$  GeV we include an additional check that demonstrates that the fit is stable when the f-5 and f-

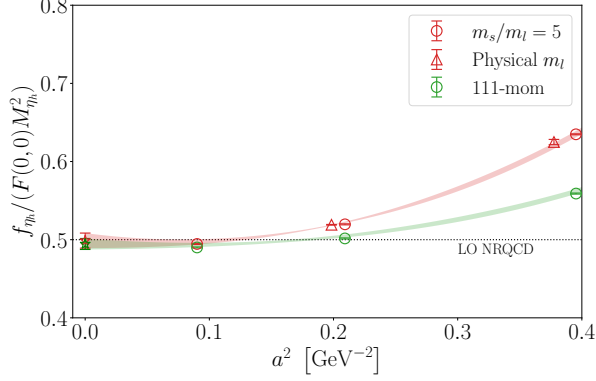

FIG. 4. Plot combining the results for the two momentum setups for  $M_{\eta_b} = 4$  GeV. The red points and band correspond to our choice of momentum in the  $y$ -direction only, and the green points and band to the case where the same total momentum is distributed evenly across the spatial dimensions (labelled ‘111-mom’). The stars in their corresponding colours are the results in the chiral/continuum limit and show excellent agreement between the two momentum setups.

phys ensembles, which have particularly large values of the lattice mass, are excluded. We show the stability plots for the  $M_{\eta_b} = 6.62$  GeV and  $M_{\eta_b} = 4$  GeV cases in Figures 6 and 7 respectively.

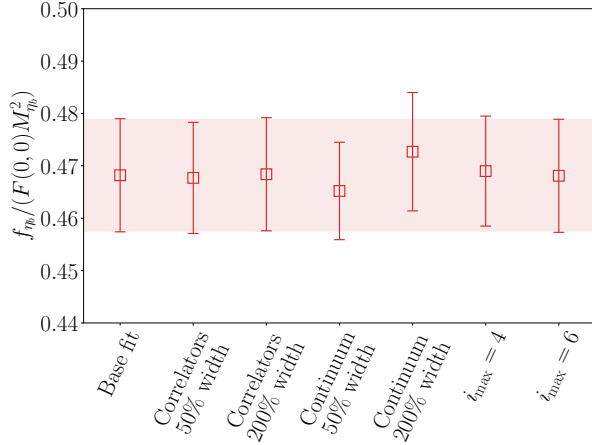

FIG. 5. Stability plot for  $R_{\eta_b}$  in the chiral/continuum limit after making variations to our base fit shown by the leftmost point and red band. From left to right we halve and double the prior widths on the parameters in the correlator fits on each of the datasets simultaneously, double and halve the prior widths for the parameters in the chiral/continuum fit, and drop and include an additional discretisation term in the fit.

The decay width  $\Gamma(\eta_b \rightarrow \gamma\gamma) = 0.557(32)_{\text{fit}}(1)_{\text{sys}}$  keV from our calculation can be combined with branching fractions determined from potential NRQCD (pNRQCD) to determine the full  $\eta_b$  width. The authors of [10] use two approaches and we make a determination from each. Combining our results with their value

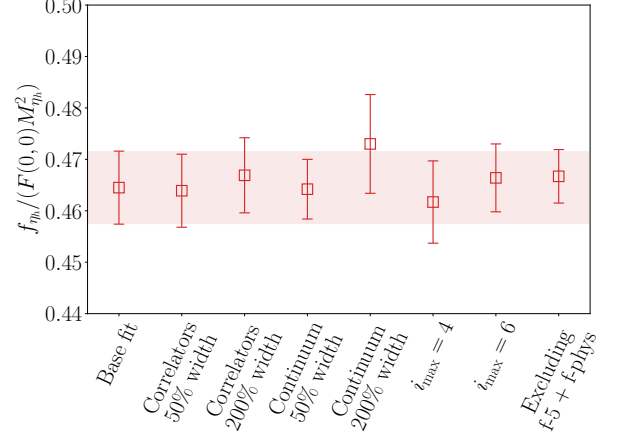

FIG. 6. Stability plot for  $R_{\eta_b}$  for  $M_{\eta_b} = 6.62$  GeV in the chiral/continuum limit after making variations to our base fit shown by the leftmost point and red band. From left to right we halve and double the prior widths on the parameters in the correlator fits on each of the datasets simultaneously, double and halve the prior widths for the parameters in the chiral/continuum fit, and drop and include an additional discretisation term in the fit. For the final point, we drop the f-5 and f-phys ensembles.

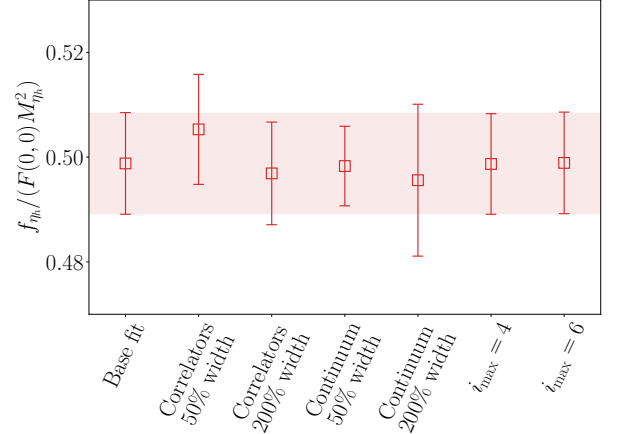

FIG. 7. Stability plot for  $R_{\eta_b}$  for  $M_{\eta_b} = 4$  GeV in the chiral/continuum limit after making variations to our base fit shown by the leftmost point and red band. From left to right we halve and double the prior widths on the parameters in the correlator fits on each of the datasets simultaneously, double and halve the prior widths for the parameters in the chiral/continuum fit, and drop and include an additional discretisation term in the fit.

from the naive non-abelianisation (NNA) method we obtain  $\Gamma(\eta_b) = 12.92^{(+45)}_{(-50)} \text{pNRQCD}(74)_{\text{LQCD}}$  MeV where the first error is from the pNRQCD calculation and the second comes from our lattice QCD result. Using the background-field gauge (BFG) method gives  $\Gamma(\eta_b) = 13.42^{(+50)}_{(-56)} \text{pNRQCD}(80)_{\text{LQCD}}$  MeV. Both numbers are in agreement with the current experimental average  $\Gamma(\eta_b) = 10^{+5}_{-4}$  MeV [3] but are much more accurate.

We summarise this comparison in Figure 8.

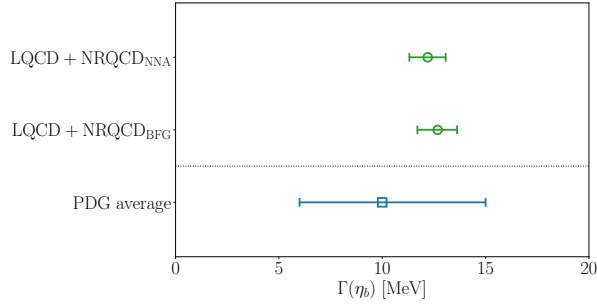

FIG. 8. Comparison of the total  $\eta_b$  width from theory and the experimental average. The green points combine our lattice QCD result for  $\Gamma(\eta_b \rightarrow \gamma\gamma)$  with the branching fraction from pNRQCD calculations in [10]. The blue point corresponds to the current experimental average [3].

[1] B. Colquhoun, L. J. Cooper, C. T. H. Davies, and G. P. Lepage (HPQCD), *Phys. Rev. D* **108**, 014513 (2023),

[arXiv:2305.06231 \[hep-lat\]](#).  
 [2] G. P. Lepage, B. Clark, C. T. H. Davies, K. Hornbostel, P. B. Mackenzie, C. Morningstar, and H. Trottier (HPQCD), *Nucl. Phys. B Proc. Suppl.* **106**, 12 (2002), [arXiv:hep-lat/0110175](#).  
 [3] S. Navas *et al.* (Particle Data Group), *Phys. Rev. D* **110**, 030001 (2024).  
 [4] D. Hatton, C. Davies, B. Galloway, J. Koponen, G. Lepage, and A. Lytle (HPQCD), *Phys. Rev. D* **102**, 054511 (2020), [arXiv:2005.01845 \[hep-lat\]](#).  
 [5] A. Bazavov *et al.* (Fermilab Lattice, MILC), *Phys. Rev. D* **98**, 074512 (2018), [arXiv:1712.09262 \[hep-lat\]](#).  
 [6] B. Chakraborty, C. T. H. Davies, B. Galloway, P. Knecht, J. Koponen, G. C. Donald, R. J. Dowdall, G. P. Lepage, and C. McNeile (HPQCD), *Phys. Rev. D* **91**, 054508 (2015), [arXiv:1408.4169 \[hep-lat\]](#).  
 [7] E. McLean, C. T. H. Davies, A. T. Lytle, and J. Koponen (HPQCD), *Phys. Rev. D* **99**, 114512 (2019), [arXiv:1904.02046 \[hep-lat\]](#).  
 [8] R. J. Dowdall, C. T. H. Davies, G. P. Lepage, and C. McNeile (HPQCD), *Phys. Rev. D* **88**, 074504 (2013), [arXiv:1303.1670 \[hep-lat\]](#).  
 [9] A. Bazavov *et al.* (Fermilab Lattice, MILC, TUMQCD), *Phys. Rev. D* **98**, 054517 (2018), [arXiv:1802.04248 \[hep-lat\]](#).  
 [10] N. Brambilla, H. S. Chung, and J. Komijani, *Phys. Rev. D* **98**, 114020 (2018), [arXiv:1810.02586 \[hep-ph\]](#).
